# Supplementary material for: Variational approach to closure of nonlinear dynamical systems: Autonomous case
Source: arXiv:1912.00394 ancillary file (2019-12-01)
Supplement: Supplementary file 1 [file Closure_CM_Supplementary_Material.pdf]

# SUPPLEMENTARY MATERIAL FOR "VARIATIONAL APPROACH TO CLOSURE OF NONLINEAR DYNAMICAL SYSTEMS: AUTONOMOUS CASE"

MICKAËL D. CHEKROUN, HONGHU LIU, AND JAMES C. MCWILLIAMS

Contents

1. Invariant manifold reduction: Applications and going beyond small spectral gap limitations 1
1.1. Application to an El Niño-Southern Oscillation (ENSO) toy model 2
1.2. Beyond invariant manifold reduction: Small spectral gaps and breakdown of slaving principles 6
2. Lower bounds of minimal dimension for exact slaving 9
References 11

Formulas or equations from the Main Text are referred below by citing their equation numbers preceded by the corresponding section they belong to. They appear in blue. The formulas or equations from this Supplementary Material are simply referred by their equation numbers. The latter appear in red.

## 1. Invariant manifold reduction: Applications and going beyond small spectral gap limitations

In this section we report on applications of the invariant manifold approximation formulas revisited in Part I. The ODE system chosen is obtained from an El Niño-Southern Oscillation (ENSO) model which exhibits a subcritical Hopf bifurcation. The purpose is to illustrate that these formulas allow for the efficient derivation of reduced systems able to capture such a bifurcation. The reason underlying this success is without any surprise contingent upon the parameter regime choice here, which, roughly speaking corresponds to a situation for which slaving (or "almost slaving") relationships hold.

Noteworthy is that this dynamical reduction is valid in practice without restriction to solutions with (exaggeratedly) small amplitudes, as it is often misleadingly believed when local invariant manifold theory is applied. We conclude this section by a discussion (Sec. 1.2 below) in which we outline natural ideas aimed at proposing meaningful parameterizations when slaving relationships are not expected to hold, and further developed in Part II of the Main Text. There, we also emphasize how the pullback limit (2.33) of Theorem 1 used to represent solutions to the homological equation Eq. (2.27) constitutes a key element for generalizing the approximation formulas of Theorem 2 beyond criticality, when slaving is violated.

*Date*: December 1, 2019.

1.1. **Application to an El Niño-Southern Oscillation (ENSO) toy model.** We recall that Suarez-Schopf model of ENSO is given by the following delay differential equation (DDE)

$$\frac{\mathrm{d}T}{\mathrm{d}t} = T(t) - \alpha T(t-\tau) - T^3(t), \tag{1}$$

where $\tau$ and $\alpha$ are positive constants; and the physically relevant range of $\alpha$ used in [SS88] is $(0,1)$. We refer to [SS88] for the physical interpretation of this model in relationship with the ENSO phenomenon, and to [NBH+98, CGN18] and references therein for other ENSO models with delays. The delay parameter $\tau$ here should not be confused with the backward integration time of the auxiliary backward-forward system considered in Part II of the Main Text.

It is clear that for this given range of $\alpha$, Eq. (1) admits three fixed points:

$$T_0 = 0, \qquad T_+ = \sqrt{1-\alpha}, \qquad T_- = -\sqrt{1-\alpha}.$$

As pointed out in [SS88], the trivial steady state is always unstable for this parameter range, whereas the stability of the two nontrivial steady states $T_\pm$ depends on $\alpha$: when $\alpha$ lies in $(0, 0.5)$ they are both locally stable for any $\tau > 0$, and when $\alpha$ lies in $(0.5, 1)$ there exists a critical $\tau$ (depending on $\alpha$) beyond which the steady states $T_\pm$ become unstable. In the following, we focus on the bifurcation arising from $T_+$ with $\tau$ as control parameter, for $\alpha$ set to a fixed value in $(0.5, 1)$ as $\tau$ is varied. The bifurcation arising from $T_-$ is of same nature, as Eq. (1) is invariant under the change of variables $T \to -T$.

For the sake of this bifurcation analysis, we introduce the perturbed variable with respect to the positive steady state, $T_+$, namely

$$u = T - T_+. \tag{2}$$

Equation (1), when written in the perturbed variable $u$, reads

$$\frac{\mathrm{d}u}{\mathrm{d}t} = (1 - 3T_+^2)u(t) - \alpha u(t-\tau) - 3T_+ u^2(t) - u^3(t). \tag{3}$$

We apply now to this equation the rigorous, the ODE approximation technique of DDEs introduced in [CGLW16], and refer to this article for the mathematical foundations and main formulas. The approach allows for efficient low-order ODE approximation of DDEs via simple analytic formulas; see [CGLW16, Sections 5-6 and Appendix C] and also [CKL18, Sec. 4.2]. By applying these formulas, setting $\alpha = 0.75$ (thus $T_+ = \sqrt{1-\alpha} = 0.5$) and the reduced dimension to be $N = 6$, the following six-dimensional ODE approximation of Eq. (3) is obtained

$$\frac{\mathrm{d}y}{\mathrm{d}t} = \left(M_1 + \frac{1}{\tau}M_2\right) y - \left(\sum_{n=1}^{6} y_n\right)^2 \left(3T_+ + \sum_{n=1}^{6} y_n\right) \left(\frac{1}{\|\mathcal{K}_0\|_{\mathcal{E}}^2}, \cdots, \frac{1}{\|\mathcal{K}_5\|_{\mathcal{E}}^2}\right)^{\mathrm{tr}}, \tag{4}$$

where $\|\mathcal{K}_n\|_{\mathcal{E}}$ denotes the norm of the underlying Koornwinder polynomials[1], which is given by (see. [CGLW16, Eq. (3.10)])

$$\|\mathcal{K}_n\|_{\mathcal{E}} = \sqrt{\frac{(n^2+1)((n+1)^2+1)}{(2n+1)}}, \qquad n \in \mathbb{N}.$$

[1]Used in [CGLW16] as basis functions to derive Galerkin approximations of DDE solutions.

Here $y = (y_1, \cdots, y_6)^{\mathrm{tr}}$, and the matrices $M_1$ and $M_2$ in (4) are respectively given by

$$M_1 = \begin{pmatrix} -0.25 & 1.25 & -2.5 & 5 & -7.75 & 11.75 \\ -0.15 & 0.75 & -1.5 & 3 & -4.65 & 7.05 \\ -0.05 & 0.25 & -0.5 & 1 & -1.55 & 2.35 \\ -0.0206 & 0.1029 & -0.2059 & 0.4118 & -0.6382 & 0.9676 \\ -0.0102 & 0.0509 & -0.1018 & 0.2036 & -0.3156 & 0.4785 \\ -0.0057 & 0.0286 & -0.0572 & 0.1143 & -0.1772 & 0.2687 \end{pmatrix}, \tag{5}$$

and

$$M_2 = \begin{pmatrix} 0 & 2 & -3 & 7 & -10 & 16 \\ 0 & -1.2 & 7.8 & -10.2 & 20.4 & -26.4 \\ 0 & -0.4 & -2.4 & 11.6 & -12.2 & 24.2 \\ 0 & -0.1647 & -0.9882 & -3.4588 & 14.7412 & -13.0941 \\ 0 & -0.0814 & -0.4887 & -1.7104 & -4.4796 & 17.7557 \\ 0 & -0.0457 & -0.2744 & -0.9605 & -2.5156 & -5.4886 \end{pmatrix}. \tag{6}$$

Numerical simulations show that over the range of $\tau$-values considered hereafter, the 6D ODE system (4) provides an excellent approximation of the DDE model (3) (not shown), and is therefore preferred since more amenable to analysis than the DDE (3). When $\alpha$ lies in the range $(0.5, 1)$, the trivial steady state $u = 0$ of Eq. (3) (equivalently $T_+$ for Eq. (1)) loses stability when the delay parameter $\tau$ crosses a critical value $\tau_c$ from above and the dynamics undergoes a subcritical Hopf bifurcation with the emergence of an unstable periodic orbit that bifurcates from 0; see Fig. 1.

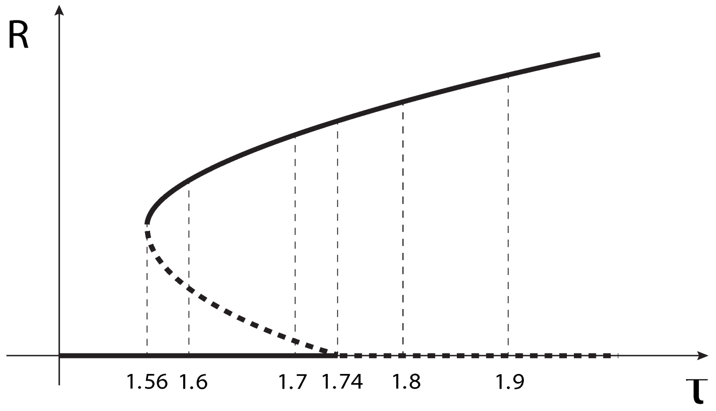


FIGURE 1. A schematic sketch of the amplitudes of the stable/unstable periodic solutions associated with Eq. (4) (and also Eq. (3)) for $\alpha = 0.75$. For this parameter value of $\alpha$, there is a subcritical Hopf bifurcation at $(y, \tau) = (0, \tau_c)$ with $\tau_c \approx 1.74$.

The ODE system (4) can be written into the following abstract equation

$$\frac{\mathrm{d}y}{\mathrm{d}t} = Ay + G(y), \tag{7}$$

with $A = M_1 + \frac{1}{\tau} M_2$, and $G$ corresponding to the nonlinear terms in (4). Our aim is to reduce this 6D system of ODEs to a lower dimensional system of ODEs not only able to capture the aforementioned subcritical Hopf bifurcation as the parameter $\tau$ is varied, but also able to capture the amplitude as well as the nonlinear features of the oscillations emerging through this bifurcation for the original system (4).

Given the spectral elements of $A$, and $E_{\mathfrak{c}}$ to be spanned by the first $m$ eigenvectors, $\boldsymbol{e}_1, \cdots, \boldsymbol{e}_m$, of the matrix $A$, we consider the parameterization $\Phi$ given by (2.68) and the associated abstract reduced equation:

$$\frac{\mathrm{d}z}{\mathrm{d}t} = A_{\mathfrak{c}} z + \Pi_{\mathfrak{c}} G\big(z + \Phi(z)\big), \tag{8}$$

where $z$ is aimed at approximating $\Pi_{\mathfrak{c}} y$; $y$ denoting the solution to Eq. (7).

By projecting the system (4) against each of the eigenvectors $\boldsymbol{e}_1, \cdots, \boldsymbol{e}_m$ of $A$, we obtain a system of equations whose components are given by:

$$\frac{\mathrm{d}z_i}{\mathrm{d}t} = \beta_i z_i + \Big\langle G\Big(\sum_{j=1}^{m} z_j \boldsymbol{e}_j + \Phi(\sum_{j=1}^{m} z_j \boldsymbol{e}_j)\Big), \boldsymbol{e}_i^*\Big\rangle, \;\; i = 1, \cdots, m, \tag{9}$$

where $z_i = \langle z, \boldsymbol{e}_i^* \rangle$, and $\langle \cdot, \cdot \rangle$ denotes the inner product on $\mathbb{C}^N$ defined in (2.46) for which $N = 6$, here.

The first pair of complex eigenvalues crosses the imaginary axis for $\tau_{\mathfrak{c}} \approx 1.74$, whereas the two other pairs stay within the left half plane even for $\tau$ well above the critical value. We choose thus $m = 2$ and the subspaces $E_{\mathfrak{c}}$ and $E_{\mathfrak{s}}$ as follows:

$$E_{\mathfrak{c}} = \mathrm{span}\{\boldsymbol{e}_1, \boldsymbol{e}_2\}, \qquad E_{\mathfrak{s}} = \mathrm{span}\{\boldsymbol{e}_3, \cdots, \boldsymbol{e}_6\}. \tag{10}$$

Setting $m = 2$ and $N = 6$ in (2.68), we obtain the following 2D reduced system:

$$\frac{\mathrm{d}z_i}{\mathrm{d}t} = \beta_i(\tau) z_i + \langle G(z_1 \boldsymbol{e}_1 + z_2 \boldsymbol{e}_2 + \Phi(z_1, z_2)), \boldsymbol{e}_i^* \rangle, \; i = 1, 2. \tag{11}$$

The numerical results are shown in Fig. 2, for the perturbed variable $u$ given by (2). Following [CGLW16, Sec. 6], $u(t)$ is reconstructed from the solution to Eq. (4) according to

$$u(t) = \sum_{j=1}^{6} y_j(t). \tag{12}$$

We denote by $\Phi_n$, the $n^{\mathrm{th}}$ component of $\Phi$. Note that

$$v(t) = z_1(t)\boldsymbol{e}_1 + z_1(t)\boldsymbol{e}_1 + \sum_{n=3}^{6} \Phi_n(z_1(t), z_2(t))\boldsymbol{e}_n \tag{13}$$

is aimed at approximating $y(t)$ solving Eq. (4). Then similarly to (12) we obtain the following approximation of $u(t)$,

$$u^{\mathrm{app}}(t) = \sum_{j=1}^{6} v_j(t) = \sum_{j=1}^{6} \Big( z_1(t)\boldsymbol{e}_1^j + z_2(t)\boldsymbol{e}_2^j + \sum_{n=3}^{6} \Phi_n(z_1(t), z_2(t))\boldsymbol{e}_n^j \Big), \tag{14}$$

where $\boldsymbol{e}_\ell^j$ denotes the $j^{\mathrm{th}}$ component of the eigenvector $\boldsymbol{e}_\ell$ for $1 \leq \ell \leq 6$.

As shown in Fig. 2, the 2D reduced system (11) allows (based on (14)) for excellent approximations of both the stable and unstable periodic limit cycles of the 6D system of ODEs (4), emerging through the aforementioned subcritical Hopf bifurcation. This is even the case for parameter values of $\tau$ relatively far from the critical value $\tau_c$ and for which the solutions' amplitude gets large.

The reason behind these good approximation skills from the reduced system (11) relies on the fact that the periodic solutions to (4) sit very close (almost slaved) to the manifold given by $\Phi$ for all the $\tau$-values shown in Fig. 2, even though the amplitude of $u$ is of order one; see Fig. 3 for a visualization of the manifold $\Phi$ along with its parameterization quality for $\tau = 1.9$, which corresponds to the furthest value to $\tau_c$ among the examined $\tau$-values.

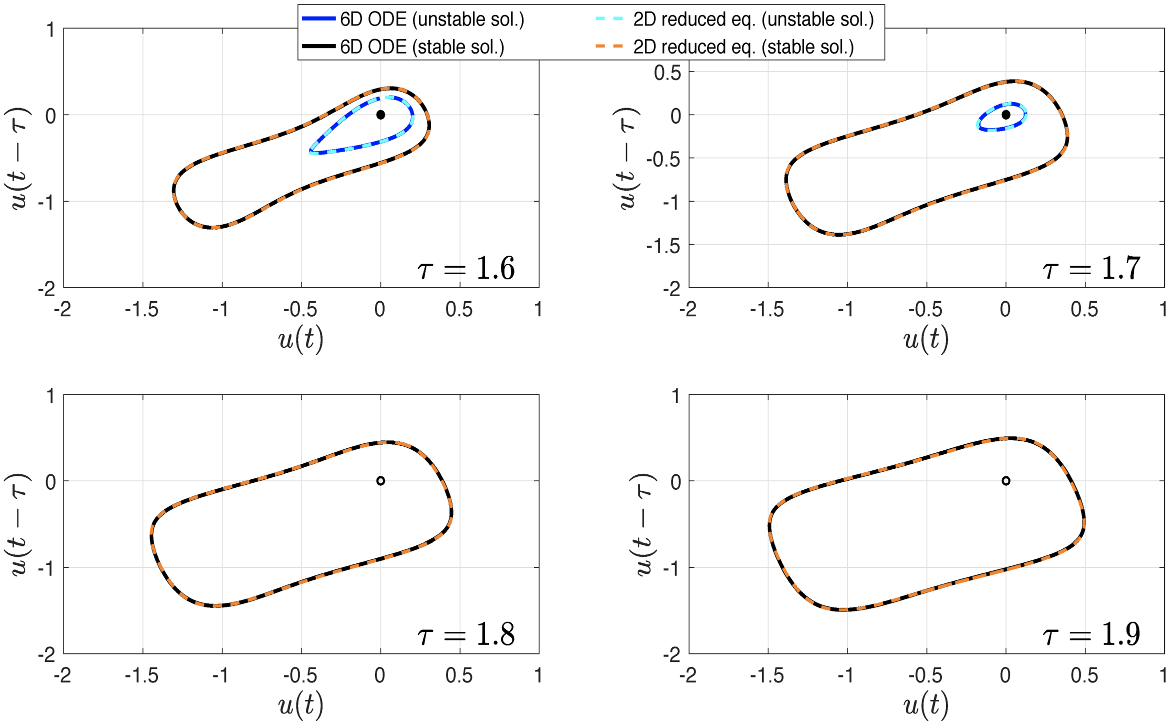


FIGURE 2. **Stable and unstable periodic solutions to the 6D Eq.** (4) **and from the 2D reduced Eq.** (11)**.** These solutions are shown using delayed coordinates $(u(t), u(t-\tau))$, with $u$ given by (12) for Eq. (4), and by (14) for Eq. (11). The value for the delay parameter $\tau$ is given in the lower right corner of each panel. In each panel, the stable (resp. unstable) periodic solution to the 6D original Eq. (4) is shown by a black (resp. blue) plain line, and the stable (resp. unstable) periodic solution to the 2D reduced Eq. (11) is shown by an orange (resp. cyan) dashed line.

To obtain Fig. 3 we represented the following norm of the manifold function $\Phi$,

$$\psi : (z_1, z_2) \mapsto \|\Phi(z_1, z_2)\|_{\mathfrak{s}}, \tag{15}$$

as a function of $\mathrm{Re}(z_1)$ and $\mathrm{Im}(z_1)$, where

$$\|w\|_{\mathfrak{s}} = \sqrt{\sum_{j=3}^{6} \left|\langle w, \boldsymbol{e}_j^* \rangle\right|^2}, \text{ for any } w \in E_{\mathfrak{s}}. \tag{16}$$

The representation of $\psi$ as a function of $\mathrm{Re} z_1$ and $\mathrm{Im} z_1$ is made possible since $E_{\mathfrak{c}}$ is spanned by eigenvectors that form a complex conjugate pair. The resulting surface, $(\mathrm{Re}(z_1), \mathrm{Im}(z_1)) \mapsto \psi(\mathrm{Re}(z_1), \mathrm{Im}(z_1))$, is then intercepted by two vertical planes for a better visual inspection of the distance between the stable periodic trajectory from Eq. (4) and this surface. The left and right panels of Fig. 3 show the curves (in red) obtained as cross sections with, respectively, the vertical plane corresponding to $\mathrm{Re}(z_1) \equiv 0$, and that corresponding to $\mathrm{Im}(z_1) = a\,\mathrm{Re}(z_1) + b$, with $a = -0.63$ and $b = 0.21$. The intersections between these planes and the stable periodic solution $P(t)$ to Eq. (4) are shown by black dots in each panel. In each case, these intersection points are very close to the graph of the mapping $\psi$ given by (15), indicating that $P(t)$ itself lies close the manifold $\Phi$ obtained by the formula (2.68), and showing thus the relevance of this parameterization.

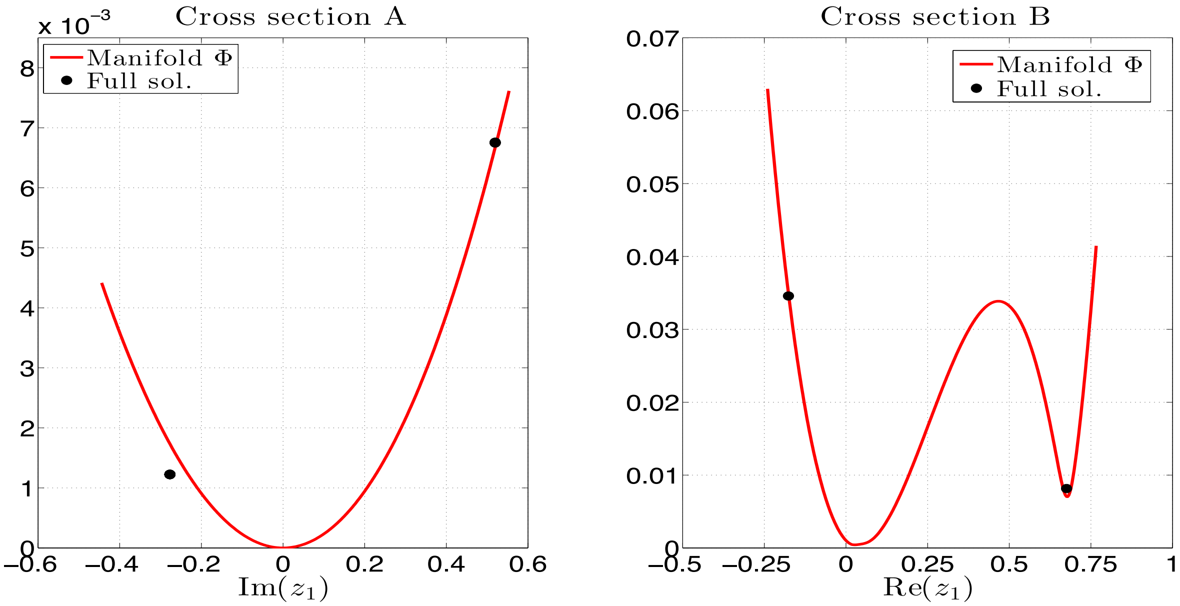


FIGURE 3. **Visualization of the manifold $\Phi$.** The curves (in red) are obtained as intersections between the graph of $\psi$ given by (15) with, respectively, the vertical plane corresponding to $\mathrm{Re} z_1 \equiv 0$ (cross section A), and that corresponding to $\mathrm{Im} z_1 = a\,\mathrm{Re} z_1 + b$ with $a = -0.63$ and $b = 0.21$ (cross section B). The black dots correspond to the intersection points of the stable periodic orbit to Eq. (4) with these vertical planes.

It is noteworthy to emphasize that the good parameterization of the stable periodic solution to Eq. (4) by the manifold $\Phi$ is not limited to these two cross sections. The quality of the parameterization can be assessed by inspecting for instance the following parameterization defect

$$R_\Phi(t) = \Phi(P_1(t), P_2(t)) - P_{\mathfrak{s}}(t),$$

where $P_j$ denotes the projection of stable periodic solution $P(t)$ to Eq. (4) onto $\boldsymbol{e}_j$ ($j = 1, 2$), while $P_{\mathfrak{s}}(t)$ denotes the projection of $P(t)$ onto $E_{\mathfrak{s}} = \mathrm{span}\{\boldsymbol{e}_3, \cdots, \boldsymbol{e}_6\}$. For the case shown in Fig. 3 ($\tau = 1.9$), the time-averaged over one period of the ratio, $\|R_\Phi(t)\|_{\mathfrak{s}}^2 / \|P_{\mathfrak{s}}(t)\|_{\mathfrak{s}}^2$, is approximately equal to $2.5 \times 10^{-2}$, indicating that $P(t)$ is almost slaved to the manifold $\Phi$. This observation explains that the discrepancies observed in Fig. 3 between the original system's solution and the manifold $\Phi$ do not affect the approximation skills of the reduced system (11) shown in Fig. 2; the fraction of the energy contained in the parameterized modes being small compared to that contained in the resolved ones. As explained in Sec. 3 of the Main Text, the usage of such parameterization defects will not only be used to diagnose the quality of a parameterization but also to design parameterizations, especially when breakdown of slaving occurs.

1.2. **Beyond invariant manifold reduction: Small spectral gaps and breakdown of slaving principles.** As mentioned in the Introduction of the Main Text and illustrated in Sec. 1.1 above, the invariant manifold reduction is a viable dimension reduction technique in situations for which slaving relationships, between the resolved and unresolved variables, hold, up to a small possible error. In such situations, the formulas of Theorem 2 given in the Main Text, or their higher-order version (see Sec. 2.3 therein), provide often efficient parameterizations. As pointed out in the Introduction, slaving relationships although more likely to occur when

the ODE dynamics is relatively simple, such as periodic or quasi-periodic, are not guaranteed to take place. Even more so, the breakdown of slaving relationships has a tendency to be encountered more often and more pronounced as bifurcation parameters are pushed towards the onset of chaos, and beyond; see [CLM17] and Sec. 3.4 of the Main Text for an example. To build intuition about this phenomenon it is useful to bear in mind that the local exponential tracking property alone, satisfied by a broad class of (local) invariant manifolds, is not strong enough to act against the breakdown of slaving.

Essentially, the local exponential tracking property says that if a solution stays in a sufficiently small neighborhood $\mathcal{V}$ of the origin for all time, then it is attracted by the manifold at an exponential rate. For instance, the local center-unstable manifold can be shown to have this local exponential tracking property[2]. This property does not exclude the possibility for a solution initially lying in $\mathcal{V}$ to either leave this neighborhood without reentering or getting in and out from time to time. As a consequence, slaving relationships are violated once a solution exits the neighborhood $\mathcal{V}$. Depending on how frequent the solution gets in and out and how far it gets away from $\mathcal{V}$, one may be in presence of slaving relationships that are violated by an error that may sporadically inflate over time spells, or even be in presence of a complete breakdown of slaving for solutions that sit outside $\mathcal{V}$. As chaos is approached, more and more modes becoming unstable and leading typically to solutions' amplitude that grows (as energy increases), it is reasonable to expect that more and more trajectories exit $\mathcal{V}$ and thus to expect a severe violation of slaving relationships. Furthermore, along the route to chaos, the spectral gap, $\gamma_m = \mathrm{Re}(\beta_m) - \mathrm{Re}(\beta_{m+1})$, (with e.g $m$ corresponding to the number of unstable modes) tends to shrink, leading to small denominators and causing exaggeratedly large coefficients in parameterizations such as (2.47)–(2.48) arising in the approximation theory of local invariant manifold.

Thus, in such situations, the parameterizations borrowed from the local invariant manifold need to be seriously revised. This is where Theorem 1 of the Main Text plays a central role as it offers to interpret the usual leading-order approximation of the invariant manifold function given by (2.47)–(2.48) therein, as a pullback limit (2.33) built from the auxiliary backward-forward system (2.29). In this representation of approximation formulas for invariant manifolds, a free parameter emerges: the backward integration time, $\tau$, over which the system (2.29) is integrated. The pullback representation provides thus dynamically-based formulas for high-mode parameterizations (and thus manifolds), conditioned upon the choice of $\tau$.

Our approach consists then to seek for manifolds within this class of parameterizations that, although may break (i) and (ii) associated with the definition of local invariant manifolds in Sec. 2.1 of the Main Text, are still meaningful in the sense that the dynamics stay nearby in a least-square sense. We propose thus in Part II of the Main Text to select this manifold in an optimal sense by minimization of a natural *parameterization defect*; see Definition 1 and (3.4) therein. Exploiting the dynamically-based formulas for our parameterizations obtained by finite-time integration of the backward-forward system (2.29), we are then left with solving a simple minimization problem in the *scalar variable*, $\tau$, only; see Sec. 4 therein. From a practical viewpoint, the dynamically-based content of our parameterizations preserves us to rely on an excessively large amount of training data in the temporal direction, as it would occur when the

[2]The local exponential tracking property is a direct consequence of the asymptotic completeness of the corresponding global invariant manifold for a modified version of the equation where the nonlinearity is multiplied by a cutoff function that vanishes outside a sufficiently small neighborhood of the origin. The interested readers are referred to [CLW15, Thm. 4.3] for conditions to ensure (global) asymptotic completeness. The proof therein was carried out for stochastic evolution equations subject to linear multiplicative noise, which can be applied to the current context by simply setting the noise strength to zero. See also [Van89, Thm. 5.17] for the derivation of the local exponential tracking property in the particular case of local center manifold.

dimension of the resolved subspace $E_{\mathfrak{c}}$ is large and a blind regression would be used to infer let us say a quadratic parameterizations with (many) arbitrary unknown coefficients. Indeed, in our case, the coefficients of our parameterizations possess analytical expressions subordinated only to the free scalar parameter $\tau$ (see e.g. Sec. 4.3 of the Main Text), allowing for minimization algorithms much less greedy in terms of data compared to a blind regression (see Appendix A of the Main Text).

We conclude this section by a simple analytic example illustrating some aspects of what has just been explained, in particular how to bypass the small denominator problem pointed out in the Introduction. This problem is typically encountered in invariant manifold approximation when small spectral gaps are present (see again (2.47)–(2.48)), regardless of whether the dynamics is simple or complicated. It turns out that, to seek for an optimal backward integration time $\tau$ actually helps alleviate this problem by introducing numerators balancing the small denominators present in standard parameterizations such as provided by Theorem 2 and in Sec. 2.3 of the Main Text.

In that respect, we consider the following $AB$-system:

$$\begin{aligned} \frac{\mathrm{d}A}{\mathrm{d}t} &= \nu_1 A + \gamma_1 AB, \\ \frac{\mathrm{d}B}{\mathrm{d}t} &= \nu_2 B - \gamma_2 A^2 - \alpha B^3. \end{aligned} \tag{17}$$

When $\nu_1 > 0$ and $\nu_2 < 0$, for any initial data $(A_0, B_0)$ with positive $A_0$, the solution will eventually approach the steady state given by

$$(\overline{A}, \overline{B}) = \big(\sqrt{(\nu_2 \overline{B} - \alpha \overline{B}^3)/\gamma_2},\, -\nu_1/\gamma_1\big), \tag{18}$$

assuming that both $\gamma_1$ and $\gamma_2$ are nonzero.

The goal of this exercise is to parameterize $\overline{B}$ in terms of $\overline{A}$ using the backward-forward system (2.29) by optimizing the backward integration time $\tau$. Simple calculations show that the manifold function $h^{(1)}_\tau$ in (2.30) is given in this case by:

$$h^{(1)}_\tau(A) = -\frac{\gamma_2(1 - e^{-(2\nu_1 - \nu_2)\tau})}{2\nu_1 - \nu_2} A^2. \tag{19}$$

The parameters are set as follows,

$$\nu_1 = 0.1,\ \gamma_1 = 0.05,\ \gamma_2 = 2\gamma_1,\ \alpha = 0.1.$$

We check the parameterization quality of $h^{(1)}_\tau$ for several different values of the spectral gap $\delta = 2\nu_1 - \nu_2$ by varying $\nu_2$. The $\tau$-value in (19) is chosen by optimizing the following parameterization defect (cf. (3.4))

$$Q(\tau) = \frac{|h^{(1)}_\tau(\overline{A}) - \overline{B}|^2}{|\overline{B}|^2}. \tag{20}$$

The left panel of Fig. 4 shows a few curves, $\tau \mapsto Q(\tau)$, for different values of the spectral gap $\delta$. It turns out that for this simple example, $h^{(1)}_\tau$, with the optimal $\tau$, provides always an exact parameterization of $\overline{B}$. In contrast, the leading-order approximation given by (2.47)–(2.48) and that corresponds to $h^{(1)}_\infty = -\gamma_2 A^2/(2\nu_1 - \nu_2)$, i.e. $h^{(1)}_\tau$ with $\tau = \infty$ (see Theorem 1 therein), always over-parameterizes $\overline{B}$ as shown in the right panel of Fig. 4. The over-parameterization gets worse as the spectral gap $\delta$ gets small, due to the small denominator $\delta = 2\nu_1 - \nu_2$. To the contrary, for $h^{(1)}_\tau$, this small denominator is balanced by the numerator $1 - e^{-\tau\delta}$ to achieve a minimization of $Q(\tau)$ when the optimal $\tau$ is used.

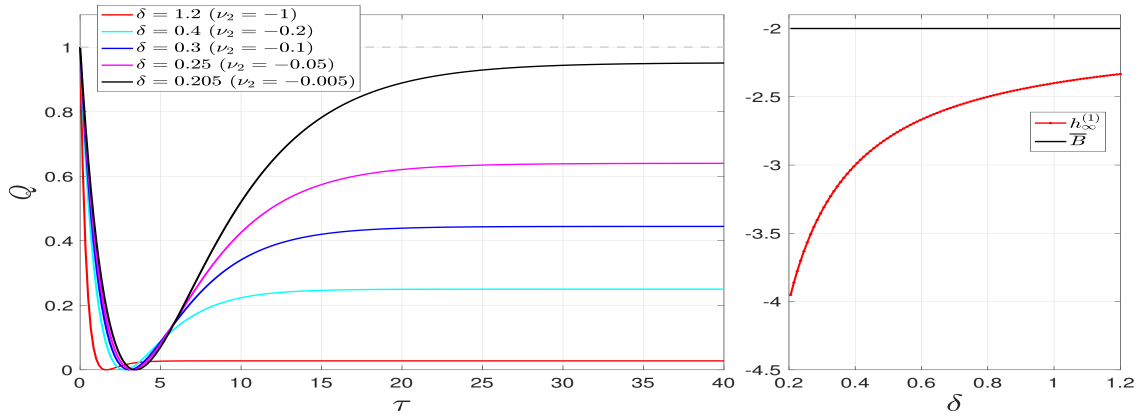


FIGURE 4. **Left panel:** Parameterization defect, $Q(\tau)$ given by (20), as $\tau$ is varied, for various values of the spectral gap $\delta = 2\nu_1 - \nu_2$. **Right panel:** $B$-component of the steady state $(\overline{A}, \overline{B})$ given by (18) as $\delta$ is varied. The parameterization, $h_\infty^{(1)}$, i.e. provided by invariant manifold theory, fails dramatically as $\delta$ is reduced.

In Sec. 3 of the Main Text, we frame within a rigorous variational approach the ideas outlined above, and in Sec. 4 of the Main Text, we provide the aforementioned general dynamically-based formulas for our parameterizations and make precise the corresponding minimization problems to solve in order to optimize them in practice.

## 2. Lower bounds of minimal dimension for exact slaving

We report in this section on the minimal reduced dimension, $m$, that guarantees the existence of an inertial manifold (IM) for the Kuramoto-Sivashinsky equation (KSE), and emphasize that the theory predicts that an IM exists when $m$ falls (far) within the dissipative range. This reduced dimension is here estimated from a *spectral gap condition (SPG)* due to [Mik91] that has been shown to provide the sharpest estimate of the minimal dimension of an inertial manifold, at least for the KSE [JRT00]. We use below this SPG to estimate a lower bound of the *minimal reduced dimension* for an IM to exist [3]. This condition applies to dissipative systems governed by the following type of parabolic equation posed in a Hilbert space $\mathcal{H}$:

$$\partial_t u + Mu = G(u), \tag{21}$$

where $M : D(M) \to \mathcal{H}$ is a linear self-adjoint operator; as usual, $D(M)$ stands for the domain of the unbounded operator $M$.

In the general case the nonlinearity $G$ diminishes the regularity; in applications this corresponds to the case in which the nonlinear terms contain spatial derivatives as for the KSE. Namely, we assume now that the nonlinearity $G$ is globally Lipschitz not as a map in $\mathcal{H}$, but as a map from $D(M^{\delta+\kappa})$ to $D(M^\kappa)$ for some $\delta \in [0, 1)$ and $\kappa \in \mathbb{R}$,

$$\|M_b^\kappa \big(G(u_1) - G(u_2)\big)\|_{\mathcal{H}} \leq \text{Lip}(G) \|M_b^{\delta+\kappa}(u_1 - u_2)\|_{\mathcal{H}}, \quad u_1, u_2 \in \mathcal{H}, \tag{22}$$

with $M_b = M + bI$ where $b = -a$ with $a$ that is chosen below.

[3]We mention also [Rom94] (not analyzed in [JRT00]) that provides similar SPG than [Mik91] in the case of the KSE; see [Zel14] for more details.

If the spectrum $\sigma(M)$ of $M$ satisfies $\sigma(M) \subset (a, \lambda] \cup [\Lambda, \infty)$ for some $\lambda$ in $(a, \Lambda)$, and $G$ satisfies the *spectral gap condition (SPG)*

$$R = \frac{\Lambda - \lambda}{(\Lambda - a)^\delta + (\lambda - a)^\delta} > \mathrm{Lip}(G), \tag{23}$$

then Eq. (21) possesses a $m$-dimensional inertial manifold with $m = \dim(\mathcal{H}_\mathfrak{c})$ where $\mathcal{H}_\mathfrak{c}$ denotes the reduced state space associated with $\sigma(M) \cap (a, \lambda]$; see [JRT00, Eq. (2.9)].

For the KSE, $M = -A = \nu \partial_x^4 + D\partial_x^2$ and one can choose $\delta = 1/4$ and $\kappa = -1/4$ as the nonlinearity maps $\mathcal{H} = L^2(0, L)$ to the Sobolev space, $H^{-1}(0, L)$, since $H^{-1}(0, L) = D(M^{-1/4})$. Within this functional setting, standard arguments give the existence and uniqueness of global solutions of the KSE given by (6.1). Nevertheless, the global Lipschitz condition does not hold for all $u_1$, $u_2$ in $\mathcal{H}$ and one typically modifies the nonlinear term in the KSE with an appropriate cutoff function that vanishes outside of an absorbing ball that contains the dynamics after transient dynamics has been removed, in order to assess whether the SPG holds or not within this absorbing ball. In this case theoretical upper bounds of $\mathrm{Lip}(G)$ can be obtained; see [JRT00].

Here, we adopt an empirical approach which consists of providing a lower bound of $\mathrm{Lip}(G)$ along a given DNS, $u(t)$, of the KSE. We place ourselves in the case considered in Sec. 6.2 of the Main Text (Regime A), i.e. for which $m \geq m_u = k_\mathfrak{c} = 31$ with $m_u$ denoting the total number of pairs of unstable modes. We selected $\Lambda = -\beta_{m+1}$, $\lambda = -\beta_m$, $a = -\beta_p - \kappa$, with $\beta_p$ corresponding to the maximum value of the eigenvalues of $A$ and where $\kappa$ is a free parameter. Given arbitrary reference points, $u_*^j = u(t_j)$ for some $t_j$ $(t_1 < \cdots < t_j < \cdots t_N)$, along the trajectory $u(t)$, the parameter $\kappa$ has been chosen so that the mapping

$$m \mapsto E_m = \frac{R_{m,\kappa}}{\max_j \max_{t \in I_j} (D_\kappa^j(t))} \tag{24}$$

has the greatest rate of growth, where

$$D_\kappa^j(t) = \frac{\| M_{\beta_p - \kappa}^{-\frac{1}{4}} \big( G(u(t)) - G(u_*^j) \big) \|_{L^2}}{\| u(t) - u_*^j \|_{L^2}}, \quad I_j = (t_j - \epsilon, t_j - \Delta t] \cup [t_j + \Delta t, t_j + \epsilon), \tag{25}$$

and where $R_m$ denotes the ratio $R$ in the SPG (23) that takes here the following form

$$R_{m,\kappa} = \frac{\beta_m - \beta_{m+1}}{(-\beta_{m+1} + \beta_p + \kappa)^{\frac{1}{4}} + (-\beta_m + \beta_p + \kappa)^{\frac{1}{4}}}. \tag{26}$$

For Regime A, we have noticed that $\kappa = 10^8$ is a good choice — based on our available data from DNS — for obtaining the smallest estimate of the *lower bound*, $m_\ell$, of the minimal reduced dimension. This lower bound is defined to be the smallest integer $m$ for which $E_m > 1$. Table 1 reports on empirical estimates of $E_m$ as $m$ is increased, for Regime A and shows that $m_\ell = 168$ for this regime.

Thus the current IM theory predicts that (exact) slaving of the high modes to the low modes, holds when the cutoff wavenumber, $k_\mathfrak{c}$, is taken sufficiently far within the dissipative range. Of course this conclusion is subject to the aforementioned SPG which is a sufficient but not a necessary condition. For instance, in the case of the KSE in Regime A, the standard QSA, $K(\xi)$ given by (4.40) of the Main Text, provides a parameterization close to slaving for a cutoff wavenumber, $k_\mathfrak{c}$, much smaller than $m = 168$.

More precisely, denoting by $\overline{(\cdot)}$ the time-average over an interval of length $T = 4$, we have that

$$\overline{\| u_\mathfrak{s}(t) - K(u_\mathfrak{c}(t)) \|_{L^2}^2} \leq \epsilon, \tag{27}$$

with $k_{\mathfrak{c}} = 48$ for $\epsilon = 0.1$ and $k_{\mathfrak{c}} = 55$, for $\epsilon = 0.01$. These numbers are found with $A = -\nu\partial_x^4 - D\partial_x^2$. Note that if $A = -\nu\partial_x^4$ as used e.g. in [JKT90], one finds $k_{\mathfrak{c}} = 55$ and $k_{\mathfrak{c}} = 65$ for $\epsilon = 0.1$ and $\epsilon = 0.01$, respectively.

However for the cutoff scale $k_{\mathfrak{c}} = 31$ considered in Sec. 6.2 of the Main Text, we have $\overline{\|u_{\mathfrak{s}}(t) - K(u_{\mathfrak{c}}(t))\|_{L^2}^2} = 2262$, due to the over-parameterization by the standard QSA already pointed out in panel (e) of Fig. 16 in the Main Text. The conclusions drawn here are further amplified for the more turbulent Regime B (not shown).

TABLE 1. Empirical estimate of the ratio $E_m$ given by (24)

| | $E_m$ | | $E_m$ |
|---|---|---|---|
| $m = 10$ | $4.3 \times 10^{-4}$ | $m = 90$ | $1.5 \times 10^{-1}$ |
| $m = 20$ | 0 | $m = 100$ | $2.1 \times 10^{-1}$ |
| $m = 30$ | $1.6 \times 10^{-4}$ | $m = 110$ | $2.8 \times 10^{-1}$ |
| $m = 31$ | $1.4 \times 10^{-3}$ | $m = 120$ | $3.7 \times 10^{-1}$ |
| $m = 40$ | $1.0 \times 10^{-2}$ | $m = 130$ | $4.7 \times 10^{-1}$ |
| $m = 50$ | $2.2 \times 10^{-2}$ | $m = 140$ | $5.8 \times 10^{-1}$ |
| $m = 60$ | $4.1 \times 10^{-2}$ | $m = 150$ | $7.2 \times 10^{-1}$ |
| $m = 70$ | $6.8 \times 10^{-2}$ | $m = 160$ | $8.8 \times 10^{-1}$ |
| $m = 80$ | $1.0 \times 10^{-1}$ | $m = 168$ | **1.02** |

## REFERENCES


[CGLW16] M. D. Chekroun, M. Ghil, H. Liu, and S. Wang, *Low-dimensional galerkin approximations of nonlinear delay differential equations*, Disc. Cont. Dyn. Sys. A **36** (2016), no. 8, 4133–4177.

[CGN18] M.D. Chekroun, M. Ghil, and J. D. Neelin, *Pullback attractor crisis in a delay differential ENSO model*, Advances in Nonlinear Geosciences (A. Tsonis, ed.), Springer, 2018, pp. 1–33.

[CKL18] M. D. Chekroun, A. Kröner, and H. Liu, *Galerkin approximations for the optimal control of nonlinear delay differential equations*, Hamilton-Jacobi-Bellman Equations. Numerical Methods and Applications in Optimal Control (D. Kalise, K. Kunisch, and Z. Rao, eds.), Berlin, Boston: De Gruyter, 2018, pp. 275–294.

[CLM17] M.D. Chekroun, H. Liu, and J.C. McWilliams, *The emergence of fast oscillations in a reduced primitive equation model and its implications for closure theories*, Computers & Fluids **151** (2017), 3–22.

[CLW15] M. D. Chekroun, H. Liu, and S. Wang, *Approximation of Stochastic Invariant Manifolds: Stochastic Manifolds for Nonlinear SPDEs I*, Springer Briefs in Mathematics, Springer, New York, 2015.

[JKT90] M. S. Jolly, I. G. Kevrekidis, and E. S. Titi, *Approximate inertial manifolds for the Kuramoto-Sivashinsky equation: Analysis and computations*, Physica D **44** (1990), no. 1, 38–60.

[JRT00] M.S. Jolly, R. Rosa, and R. Temam, *Evaluating the dimension of an inertial manifold for the Kuramoto-Sivashinsky equation*, Advances in Differential Equations **5** (2000), no. 1-3, 31–66.

[Mik91] M. Miklavčič, *A sharp condition for existence of an inertial manifold*, J. Dynam. Diff. Eqns. **3** (1991), no. 3, 437–456.

[NBH+98] J. D. Neelin, D. S. Battisti, A. C. Hirst, F.-F. Jin, Y. Wakata, T. Yamagata, and S. E. Zebiak, *ENSO theory*, Journal of Geophysical Research: Oceans (1978–2012) **103** (1998), no. C7, 14261–14290.

[Rom94] A. V. Romanov, *Sharp estimates of the dimension of inertial manifolds for nonlinear parabolic equations*, Russian Academy of Sciences. Izvestiya Mathematics **43** (1994), no. 1, 31.

[SS88] M. J. Suarez and P. S. Schopf, *A delayed action oscillator for ENSO*, J. atmos. Sci. **45** (1988), 3283–3287.

[Van89] A. Vanderbauwhede, *Centre manifolds, normal forms and elementary bifurcations*, Dynamics reported, Springer, 1989, pp. 89–169.

[Zel14] S. Zelik, *Inertial manifolds and finite-dimensional reduction for dissipative PDEs*, Proc. R. Soc. Edinb. Sec. A: Mathematics **144** (2014), no. 6, 1245–1327.

(MDC) Department of Earth and Planetary Sciences, Weizmann Institute, Rehovot 76100, Israel; and Department of Atmospheric and Oceanic Sciences, University of California, Los Angeles, CA 90095-1565, USA
*Email address*: mchekroun@atmos.ucla.edu

(HL) Department of Mathematics, Virginia Polytechnic Institute and State University, Blacksburg, Virginia 24061, USA
*Email address*: hhliu@vt.edu

(JCM) Department of Atmospheric & Oceanic Sciences, University of California, Los Angeles, CA 90095-1565, USA
*Email address*: jcm@atmos.ucla.edu
